# Supplementary material for: Robust Online Monitoring of Signal Temporal Logic
Source: arXiv:1506.08234 source file (2015-06-26)
Supplement: Supplementary file 1 [file appendix.tex]

\begin{proof}
We prove by induction on the formula structure. The base case is when
$\varphi$ is $\mu$.  If $\tau \in \signalspan(\vy)$ then
$\introb(\varphi,\vy,\tau)$ = $[f(\vy(\tau)),f(\vy(\tau))]$.  Let $\vx$ be
any completion of $\vy$. If $\tau \in \signalspan(\vy)$ then $\vx(\tau) =
\vy(\tau)$, and hence, $\inf_{\vx \in \completions(\vy)} \rob(\varphi, \vx,
\tau)$ (resp. $\sup$) is equal to $f(\vy(\tau))$. If $\tau \not\in
\signalspan(\vy)$, then $\introb(\varphi,\vy,\tau) = [\flo,\fhi]$. By
definition of $\flo$ and $\fhi$, for any completion $\vx$, $f(\vx(\tau))
\in [\flo,\fhi]$. 

We proceed by structural induction on the formula structure. Assume
$\introb(\varphi,\vy,\tau)$ is a \rsi, \ie, for any completion $\vx$ of
$\vy$, $\rob(\varphi,\vx,\tau) \in \introb(\varphi,\vy,\tau)$.  As
$\rob(\neg \varphi,\vx,\tau)$ = $-\rob(\varphi, \vx, \tau)$, it follows
that if $\rob(\varphi,\vx,\tau) \in \introb(\varphi,\vy,\tau)$, then
$-\rob(\varphi,\vx,\tau) \in -\introb(\varphi,\vy,\tau)$, by interval
arithmetic. For all the remaining operators, we can make a similar
argument, and the results follow by the properties of interval arithmetic.
\end{proof}
